# Supplementary material for: Revisiting Click-based Interactive Video Object Segmentation
Source: arXiv:2203.01784 source file (2022-06-07)
Supplement: Supplementary file 1 [file appendix.tex]

\section{Appendix}
\label{sec:appendix}

\begin{table}[h]
	\begin{center}
		\resizebox{\columnwidth}{!}{
			\begin{tabular}{lccccc}
				\hline
				\multirow{2}{*}{Method}					& \GrabCut 	         & \Berkeley	      &\DAVIS              & \SBD		        \\
														& @$0.90\downarrow$  & @$0.90\downarrow$  & @$0.90\downarrow$  & @$0.90\downarrow$  \\
				\hline
				IA+SA~\cite{kontogianni2020continuous}  & $3.07$             & $4.94$             & $-   $             & $-   $             \\
				\fBRS									& $2.46$		     & $4.65$ 		      & $8.21$             & $8.30$   	        \\
				\FCANet									& $2.08$ 		     & $3.92$ 		      & $7.57$             & $-	  $   	        \\
				\RITM									& $\mathbf{1.70}$    & $\mathbf{2.48}$    & $\mathbf{6.00}$    & $\mathbf{6.86}$    \\
				S2M~(MiVOS)~\cite{Cheng_CVPR_2021}		& $4.40$			 & $6.54$			  & $9.39$			   & $12.89$ 			\\
				\hline
			\end{tabular}
		}
	\caption{Evaluation results of~\sota iIOS methods against the S2M interaction module on popular iIOS datasets in order to find an appropriate interaction module for our click based iVOS method. Best results are achieved by RiTM as highlighted in bold.}
	\end{center}
	\label{tab_iIOS_methods}
\end{table}

\subsection{Ablation Study}
We conduct an ablation studie on the interactive DAVIS validation set, shown in~\tabref{tab_ablation}. By integrating the previous masks from both propagation and interaction into each other, the process is able to gain $0.06$ points better than without. In addition, by not relying on any threshold CiVOS performs better, which alleviates the fine-tuning of our approach.

\begin{table}[h]
	\begin{center}
		\resizebox{\columnwidth}{!}{%
		\begin{tabular}{ccccc}
			Previous mask 	& Propagation binary mask 	& Interaction binary mask 	& new aggregation 	& \AUC\J	 			\\
			\hline
			\unchecked		& \checked				& \checked				& \unchecked		& $0.64$				\\	% exp 18
			\checked		& \checked				& \checked				& \unchecked		& $0.70$				\\	% exp 07
			\checked		& \unchecked			& \checked				& \unchecked		& $0.72$				\\	% exp 08
			\checked		& \unchecked			& \unchecked			& \unchecked		& $0.73$				\\	% REDOO ALL expirement by using f2 and only one click per interaction
			\checked		& \unchecked			& \unchecked			& \checked			& $0.72$				\\
			\hline
		\end{tabular}
		}
		\caption{Ablation study on the DAVIS validation set. Clicks where extracted following the $f_{2}$ strategy, where only one click per object per round was allowed.}
	\end{center}
	\label{tab_ablation}
\end{table}
